# Supplementary material for: Fault-tolerant Fusion-based Quantum Computing with the Four-legged Cat Code
Source: arXiv:2508.03796 source file (2025-08-07)

# Standard Foliation

① Teleportation chain for each data qubit

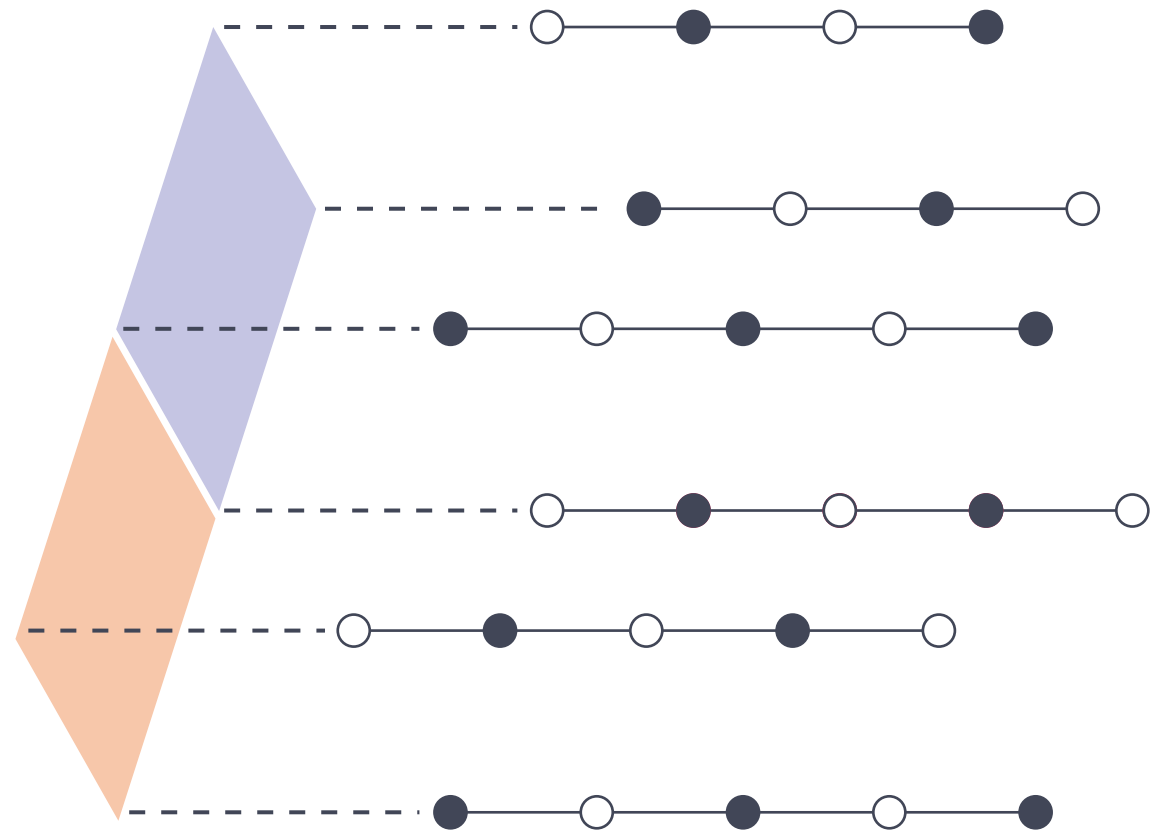

② Introduce qubits that measure the stabilizers

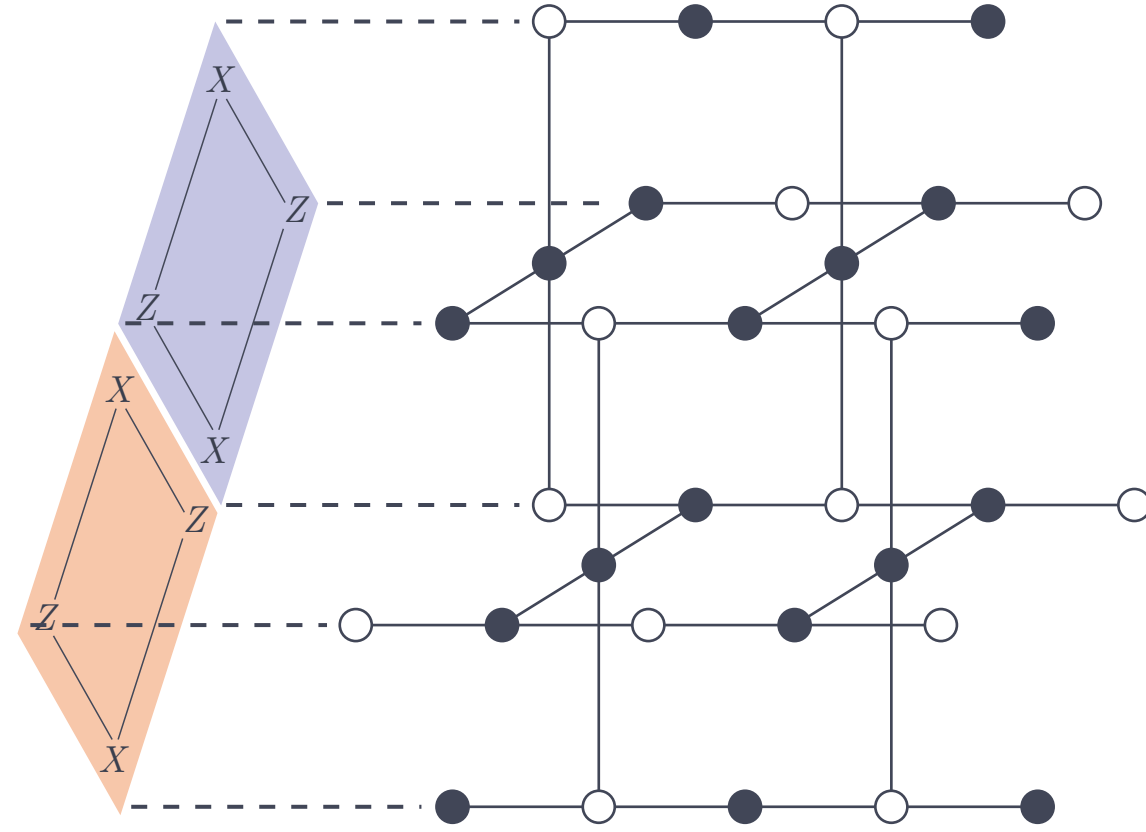

③ Split each qubit into two qubits  
These qubits are to be fused with each other

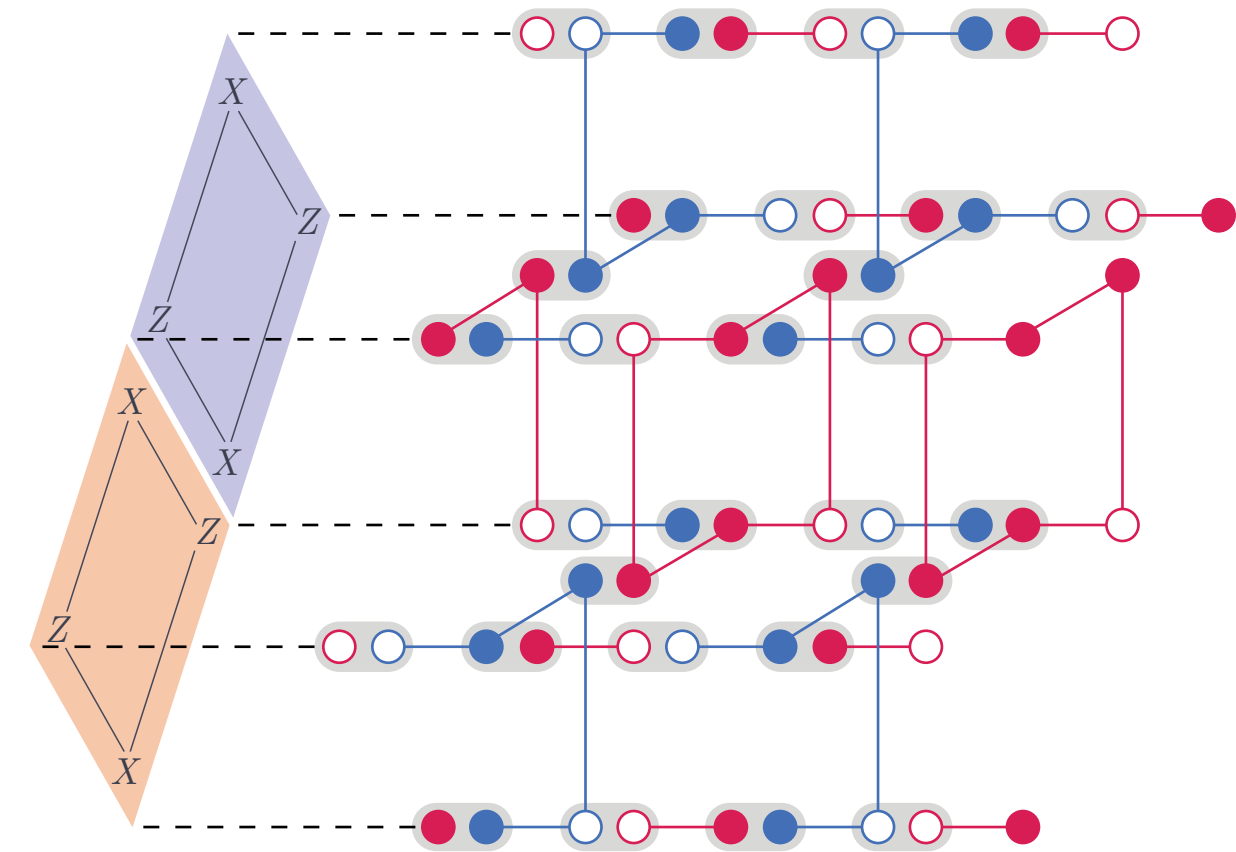

# Quasi-Planar Foliation

① Teleportation chain for each data qubit

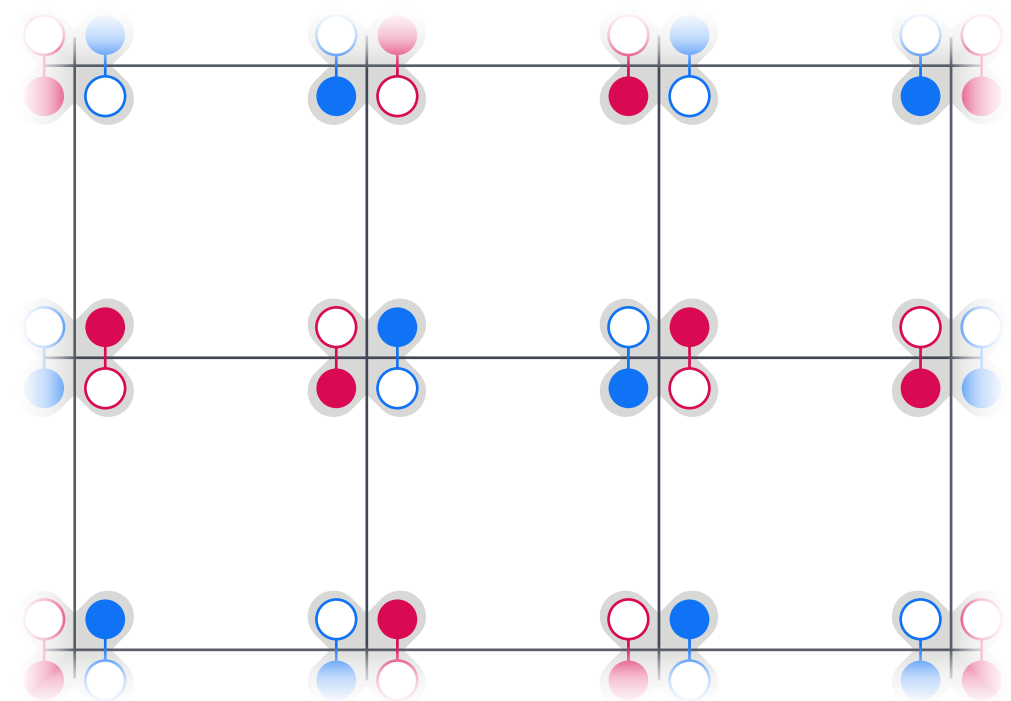

2a) Measure half the stabilizers

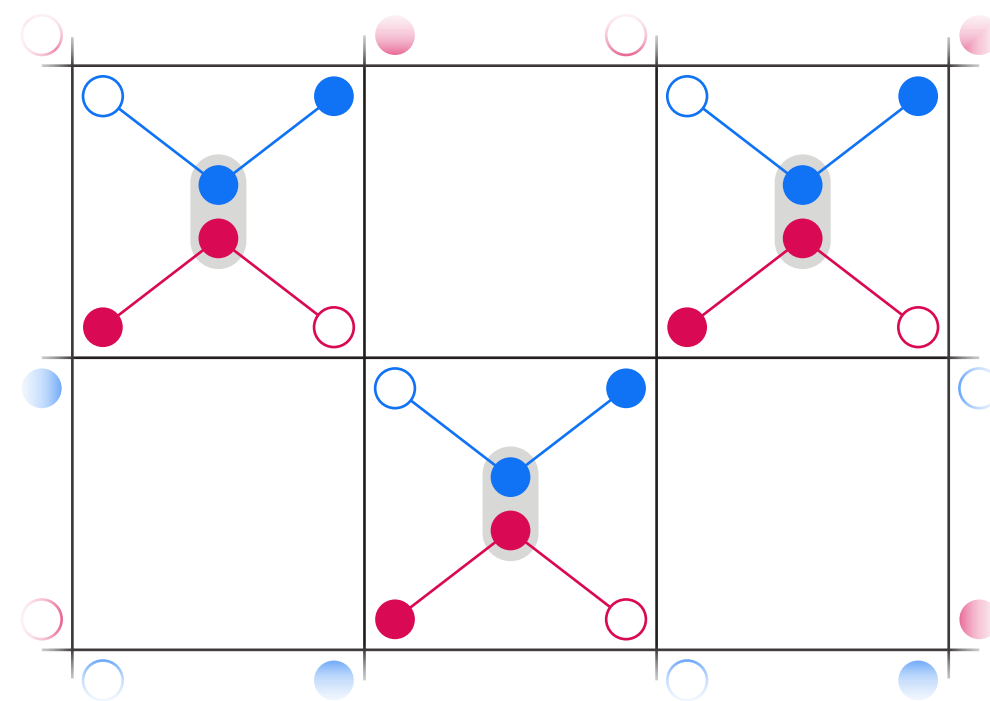

2b) Measure the other stabilizers

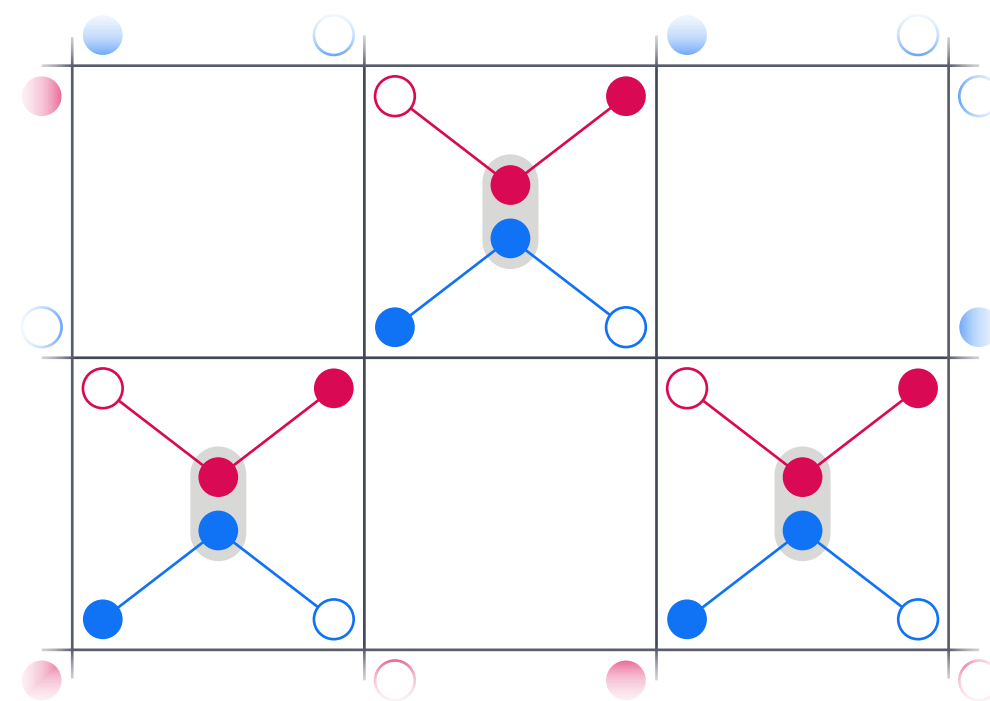

③ Unify both steps  $\Rightarrow$  six-ring planar FBEC

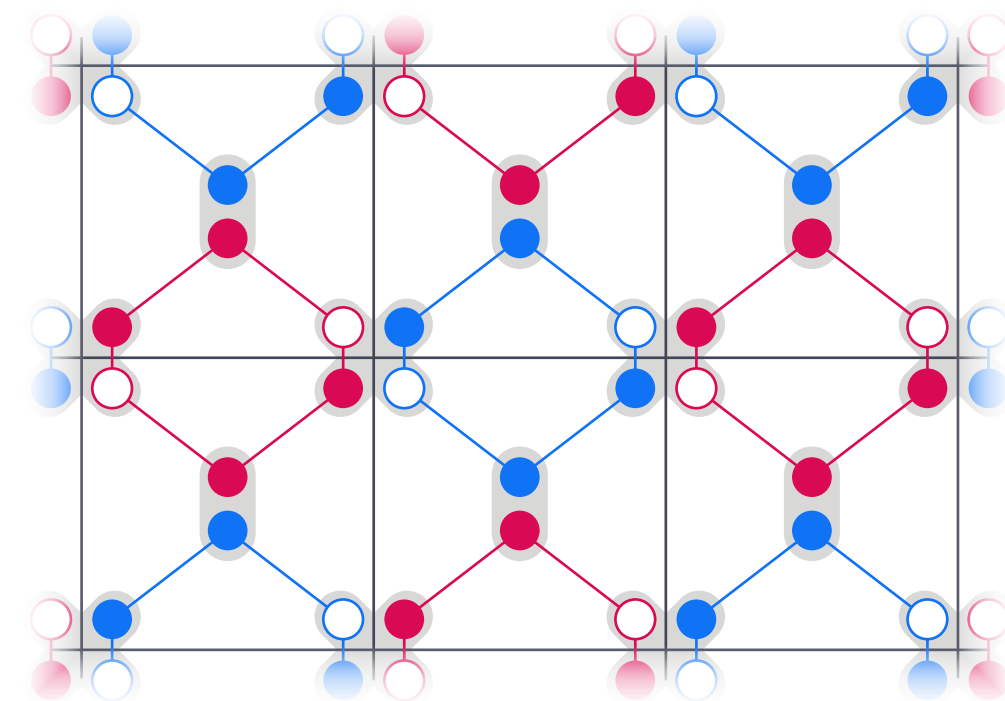

Supplement: Supplementary file 1 [file planar_foliation.pdf]
